# Supplementary material for: Exciton-Exciton Annihilation Is Coherently Suppressed in H-Aggregates, but Not in J-Aggregates
Source: arXiv:1705.05861 ancillary file (2017-05-16)
Supplement: Supplementary file 1 [file Tempelaar_SM.pdf]

# Supplemental Material for
# Exciton-Exciton Annihilation Is Coherently Suppressed in H-Aggregates, but Not in J-Aggregates

Roel Tempelaar,[1,2,*] Thomas L. C. Jansen,[1] and Jasper Knoester[1,†]

[1] *University of Groningen, Zernike Institute for Advanced Materials, Nijenborgh 4, 9747 AG Groningen, The Netherlands*

[2] *Department of Chemistry, Columbia University, 3000 Broadway, New York, New York 10027, USA*

This Supplemental Material contains an analytical derivation of the zero-temperature exciton-exciton annihilation rates for disorder-free, periodic J- and H-aggregates with nearest-neighbor couplings between the $S_0 - S_1$ transitions and point-dipoles couplings between parallel $S_0 - S_1$ and $S_1 - S_n$ transitions, taken in the long-aggregate limit. It demonstrates that under these assumptions, $\Gamma^{\mathrm{J}} \approx 4\Gamma^{\mathrm{H}}$.

Adopting a center-of-mass representation, the two-exciton eigenstates of the Hamiltonian (Eq. 4 of the main text) are expanded as

$$|\Psi_{K,q}\rangle = \sum_{m_1>m_2} c^{K,q}_{m_1,m_2}|m_1, m_2\rangle. \tag{S1}$$

Disregarding disorder (setting $\epsilon_m = 0$ for all $m$), and assuming periodic boundary conditions and nearest-neighbor couplings between $S_0 - S - 1$ transitions ($J_{m_1,m_2} = J_{\mathrm{NN}}\delta_{m_1,m_2\pm1}$), the wavefunction coefficients are given by [1]

$$c^{K,q}_{m_1,m_2} = \frac{2}{M}e^{iK\pi(m_1+m_2)/M}\sin\Big(q\pi\frac{m_1-m_2}{M}\Big), \tag{S2}$$

with the corresponding eigenenergies

$$\omega_{K,q} = 4J_{\mathrm{NN}}\cos\Big(\frac{K\pi}{M}\Big)\cos\Big(\frac{q\pi}{M}\Big), \tag{S3}$$

where $M$ denotes the number of molecules, and under the constraint that $K = 0, 2, \ldots, 2M-2$ and $q = 1, 3, \ldots, M-2$. At $T = 0$ K, the annihilation rate is given by

$$\Gamma = \frac{2\pi}{\hbar}\rho(E_{\mathrm{f}})\sum_{m=1}^{M}|\langle S_{n(m)}|H_{\mathrm{a}}|\Psi_{K_0,q_0}\rangle|^2, \tag{S4}$$

where $\Psi_{K_0,q_0}$ represents the band-bottom eigenstate. Setting $\rho(E_{\mathrm{f}}) = 1/\gamma$, and with substitution of Eq. 3 (of the main text) and Eq. S2, this expression can be recast as

$$\begin{aligned}\Gamma &= \frac{2\pi}{\hbar\gamma}\sum_{m_1=1}^{M}\Big|\sum_{m_2=1}^{m_1-1}V_{m_1,m_2}c^{K_0,q_0}_{m_1,m_2} + \sum_{m_2=m_1+1}^{M}V_{m_1,m_2}c^{K_0,q_0}_{m_2,m_1}\Big|^2\\ &= \frac{2\pi}{\hbar\gamma}\sum_{m_1=1}^{M}\Big|\sum_{m_2=1}^{M}V_{m_1,m_2}d^{K_0,q_0}_{m_1,m_2}\Big|^2,\end{aligned} \tag{S5}$$

with $d^{K_0,q_0}_{m_1,m_2} \equiv \Theta(m_1-m_2)c^{K_0,q_0}_{m_1,m_2} + \Theta(m_2-m_1)c^{K_0,q_0}_{m_2,m_1}$ representing the symmetrized wavefunction coefficients (see main text), and $V_{m_1,m_2} \equiv V_{\mathrm{NN}}/|m_1-m_2|^3$ taken in the point-dipole approximation. Making use of the translational symmetry of the linear, periodic, and

disorder-free aggregate, we can further reformulate the result as

$$\Gamma = \frac{2\pi V_{\mathrm{NN}}^2}{\hbar\gamma}\sum_{m=1}^{M}\Big|\sum_{r=-M/2+1}^{M/2}\frac{d_{m,m+r}^{K_0,q_0}}{|r|^3}\Big|^2, \tag{S6}$$

while imposing $r \neq 0$, and taking $M$ to be an even number. For J-aggregates, the band-bottom eigenstate corresponds to $K_0 = 0$ and $q_0 = 1$, so that

$$c_{m_1,m_2}^{\mathrm{J}} \equiv c_{m_1,m_2}^{0,1} = \frac{2}{M}\sin\Big(\pi\frac{m_1-m_2}{M}\Big), \tag{S7}$$

and

$$d_{m_1,m_2}^{\mathrm{J}} = \frac{2}{M}\sin\Big(\pi\frac{|m_1-m_2|}{M}\Big). \tag{S8}$$

Consequentially,

$$\Gamma^{\mathrm{J}} = \frac{8\pi V_{\mathrm{NN}}^2}{\hbar\gamma M}\Big|\sum_{r=-M/2+1}^{M/2}\frac{\sin(\pi|r|/M)}{|r|^3}\Big|^2. \tag{S9}$$

The summation over $r$ can then be rewritten as

$$\sum_{r=-M/2+1}^{M/2}\frac{\sin(\pi|r|/M)}{|r|^3} = 2\sum_{r=1}^{M/2}\frac{\sin(\pi r/M)}{r^3} - \Big(\frac{2}{M}\Big)^3. \tag{S10}$$

Upon taking the large-aggregate limit, $M \to \infty$, the second term vanishes. Further assuming $M$ to be the square of some integer value, we obtain for the first term

$$2\sum_{r=1}^{M/2}\frac{\sin(\pi r/M)}{r^3} = 2\sum_{r=1}^{\sqrt{M}}\frac{\pi r/M + \mathcal{O}(r^3/M^3)}{r^3} + 2\sum_{r=\sqrt{M}+1}^{M/2}\frac{\sin(\pi r/M)}{r^3}. \tag{S11}$$

The second term satisfies

$$|\,2\sum_{r=\sqrt{M}+1}^{M/2}\frac{\sin(r\pi/M)}{r^3}| < 2\sum_{r=\sqrt{M}+1}^{M/2}\frac{1}{r^3} < \frac{M-2\sqrt{M}-2}{(\sqrt{M}+1)^3} < \frac{1}{\sqrt{M}}, \tag{S12}$$

which also vanishes with $M \to \infty$. This leaves

$$2\sum_{r=1}^{M/2}\frac{\sin(r\pi/M)}{r^3} \approx \frac{2\pi}{M}\sum_{r=1}^{\sqrt{M}}\frac{1}{r^2} \approx \frac{\pi^3}{3M}, \tag{S13}$$

yielding for the annihilation rate

$$\Gamma^{\mathrm{J}} \approx \frac{8\pi^7 V_{\mathrm{NN}}^2}{9\hbar\gamma M^3}. \tag{S14}$$

Note that we find the same $\Gamma \propto 1/M^3$ scaling as was found in Ref. 2 for two-exciton states within a coherent domain. For H-aggregates, the band-bottom eigenstate corresponds to $K_0 = M$ and $q_0 = 1$, yielding

$$c^{\mathrm{H}}_{m_1,m_2} \equiv c^{M,1}_{m_1,m_2} = \frac{2}{M}(-1)^{(m_1+m_2)} \sin\left(\frac{m_1 - m_2}{M}\pi\right) = (-1)^{(m_1+m_2)} c^{\mathrm{J}}_{m_1,m_2}, \tag{S15}$$

and also

$$d^{\mathrm{H}}_{m_1,m_2} = (-1)^{(m_1+m_2)} d^{\mathrm{J}}_{m_1,m_2}. \tag{S16}$$

As a consequence,

$$\Gamma^{\mathrm{J}} = \frac{8\pi V_{\mathrm{NN}}^2}{\hbar\gamma M}\Big| \sum_{r=-M/2+1}^{M/2} (-1)^r \frac{\sin(\pi|r|/M)}{|r|^3} \Big|^2. \tag{S17}$$

Analogously to the J-aggregate case, the summation can be approximated as

$$\sum_{r=-M/2+1}^{M/2} (-1)^r \frac{\sin(\pi|r|/M)}{|r|^3} \approx \frac{2\pi}{M} \sum_{r=1}^{\sqrt{M}} \frac{(-1)^r}{r^2} \approx \frac{\pi^3}{6M}, \tag{S18}$$

so that the annihilation rate is given by

$$\Gamma^{\mathrm{H}} \approx \frac{2\pi^7 V_{\mathrm{NN}}^2}{9\hbar\gamma M^3}. \tag{S19}$$

Comparing Eqs. S14 and S19, it follows that $\Gamma^{\mathrm{J}} \approx 4\Gamma^{\mathrm{H}}$.

---

* r.tempelaar@gmail.com

† j.knoester@rug.nl

[1] F. C. Spano and S. Mukamel, The Journal of Chemical Physics **95**, 7526 (1991).

[2] V. Malyshev, H. Glaeske, and K.-H. Feller, Chemical Physics Letters **305**, 117 (1999).
